# Supplementary material for: Normal Form Bisimulations By Value
Source: arXiv:2303.08161 source file (2023-09-05)
Supplement: Supplementary file 2 [file toappendix.tex]

\gettoappendix {l:ss-bs-equivalence_weak}
\gettoappendix {prop:ncbv-coherence}
\gettoappendix {prop:main-lemma_naive}
\gettoappendix {prop:enf-validation-of-equivalences}
\gettoappendix {thm:cbv-scrutability-characterization}
\gettoappendix {prop:strong-bisimulation}
\gettoappendix {l:ss-bs-equivalence_vsce}
\gettoappendix {prop:substitutivity_vsce}
\gettoappendix {thm:nafex-included-leqc}
\gettoappendix {prop:type-preorder-is-compatible}
\gettoappendix {prop:bisimulation-preserves-typeder}
\gettoappendix {l:smaller-derivations-stuck}
\gettoappendix {l:enf-bisimulation-preserves-typeder}
\gettoappendix {prop:etav-for-leqtypetwo}
